# Supplementary material for: Visualizing Regulation in Rule-based Models
Source: arXiv:1509.00896 ancillary file (2015-09-02)
Supplement: Supplementary file 1 [file visualizing-regulation-rule-SUPPLEMENT.pdf]

BIOINFORMATICS

Vol. 00 no. 00 2015
Pages 1–16

# Visualizing Regulation in Rule-based Models : Supplement

John A. P. Sekar [1], Jose-Juan Tapia [1] and James R. Faeder [1*]

[1]Department of Computational and Systems Biology, University of Pittsburgh School of Medicine, Pittsburgh, PA 15260

Received on XXXXX; revised on XXXXX; accepted on XXXXX

Associate Editor: XXXXXXX

**ABSTRACT**

This supplement is provided along with the paper titled Visualizing Regulation in Rule-based Models. Sections 1-5 provide the graph theory for interconverting between graph abstractions. Section 6 contains Figures S1-S9.

**Availability:** The software implementation is available with BioNetGen 2.2.6. Documentation is available at http://bionetgen.org/.

**Contact:** faeder@pitt.edu

## 1 PRELIMINARY DEFINITIONS

1. A graph takes the form $G = (V, E)$ where $V$ is a set of vertices and $E \subset V \times V$ is a set of unordered vertex pairs.
2. We use functions to embed vertex and edge attributes. A *prototype* is a type of function and is denoted without suffixes, e.g. $f$. An *application*, e.g. $f_X$ is a specific instance of the prototype mapped over a domain $X$.
3. Two applications of the same prototype are *consistent* (denoted by $\equiv$) if they map identically on the intersection of their domains.

$$f_X \equiv f_{X'} \iff f_X(x) = f_{X'}(x), \forall x \in X \cap X'$$

4. Consistent applications preserve set relations such as subset and union.

$$\begin{aligned} &X' \subset X, f_{X'} \equiv f_X \\ &\quad \implies f_{X'}(x) = f_X(x), \forall x \in X' \\ &Z = X \cup Y, f_X \equiv f_Y, f_Z \equiv f_X, f_Z \equiv f_Y \\ &\quad \implies f_Z(x) = \begin{cases} f_X(x), & x \in X \\ f_Y(x), & x \in Y \end{cases} \end{aligned}$$

In the rest of this work, any reference to construction of a set by union or subset of other sets implies a corresponding consistency-preserving construction on any applications that have been defined on the sets involved.

$$X' \subset X \implies f_{X'} \equiv f_X$$
$$Z = X \cup Y, f_X \equiv f_Y \implies f_Z \equiv f_X, f_Z \equiv f_Y$$

5. The notation can be generalized to *sets* of function prototypes applied over a single domain. If $F$ denotes a set of prototypes, then $F_X$ is a set of applications of each prototype in $F$ to the domain $X$.

$$F = \{f | f \text{ is a prototype }\}$$
$$F_X = \{f_X, \forall f \in F\}$$

Two sets of applications are consistent, if there exists a pairwise relation preserving consistency and prototype.

$$F_X \equiv F_Y \iff f_X \equiv f_Y, \forall f \in F$$

6. A *graph type* is defined by a set of vertex function prototypes $\Lambda$ and a set of edge function prototypes $\Sigma$. An *instance* of a graph type has specific applications of $\Lambda$ on a vertex set $V$ and $\Sigma$ on an edge set $E$ respectively.

$$G = (V, E, \Lambda_V, \Sigma_E)$$

In the rest of this work, a 'graph' refers to a graph instance with appropriate node and edge applications. When one graph type is transformed to another, new node and edge applications need to be defined corresponding to the new graph type.

7. A subgraph relation (denoted by $\sqsubset$) between two graphs is a subset relation between vertices and edges with consistent vertex and edge applications.

$$\begin{aligned} &G = (V, E, \Lambda_V, \Sigma_E), \\ &G' = (V', E', \Lambda_{V'}, \Sigma_{E'}), \\ &V' \subset V, E' \subset E, \\ &\Lambda_V \equiv \Lambda_{V'}, \Sigma_E \equiv \Sigma_{E'} \\ &\quad \implies G' \sqsubset G \end{aligned}$$

8. A *trivial merge* (denoted by $\sqcup$) between two graphs is a union of vertex and edge sets that preserves consistency of the vertex and edge applications.

$$\begin{aligned} &G = (V, E, \Lambda_V, \Sigma_E), \\ &G' = (V', E', \Lambda_{V'}, \Sigma_{E'}), \\ &\Lambda_V \equiv \Lambda_{V'}, \Sigma_E \equiv \Sigma_{E'} \\ &\quad \implies G \sqcup G' = (V \cup V', E \cup E', \Lambda_{V \cup V'}, \Sigma_{E \cup E'}) \end{aligned}$$

*to whom correspondence should be addressed

© Oxford University Press 2015.

9. A *vertex remap* operation $\mathcal{VM}(v_0 \to v_1) \circ G$ copies edges incident on vertex $v_0$ to another vertex $v_1$.

$$G = (V, E, \Lambda_V, \Sigma_E)$$
$$v_0, v_1 \in V$$
$$E_v = \{(v, v') \in E | v_0 \in \{v, v'\}\}$$
$$g(v) = \begin{cases} v_1, & v = v_0 \\ v, & v \neq v_0 \end{cases}$$
$$E_{v'} = \{(g(v), g(v')), \forall (v, v') \in E_v\}$$
$$\mathcal{VM}(v_0 \to v_1) \circ G = (V, E \cup E_{v'}, \Lambda_V, \Sigma_{E \cup E'})$$

10. A *vertex remove* operation $\mathcal{VD}(v_0) \circ G$ removes a vertex from a graph and any edges incident on the vertex.

$$G = (V, E, \Lambda_V, \Sigma_E)$$
$$v_0 \in V$$
$$E_v = \{(v, v') \in E | v_0 \in \{v, v'\}\}$$
$$\mathcal{VD}(v_0) \circ G = (V - \{v_0\}, E - E_v, \Lambda_{V - \{v_0\}}, \Sigma_{E - E_v})$$

11. Operations can be linked together as sequences. The sequence $Del(X)$ deletes nodes belonging to a particular subset $X$. The order of the delete operations is immaterial.

$$Del(X) \circ G = \left\{ \prod_{v \in X} \mathcal{VD}(v) \right\} \circ G$$

The sequence $Map(Y)$ performs a series of remap operations using a set of ordered pairs of nodes $Y$.

$$Map(Y) \circ G = \left\{ \prod_{(v, v') \in Y} \mathcal{VM}(v \to v') \right\} \circ G$$

The order of the remap operations is immaterial as long as there is no overlap between the sources and targets, i.e.

$$Src \cap Tgt = \{\}$$
$$\text{where } v \in Src, v' \in Tgt, \forall (v, v') \in Y$$

12. A *filter* operation $\mathcal{F}(f, y) \circ X$ creates a subset of the domain $X$ that maps to a value $y$ under the application of the prototype $f$.

$$\mathcal{F}(f, y) \circ X = \{x \in X | f_X(x) = y\}$$

Filters can also be sequentiated. Given $Y$, a set of tuples of function prototypes and values,

$$Fil(Y) \circ X = \left\{ \prod_{(f, y) \in Y} \mathcal{F}(f, y) \right\} \circ X$$

13. We use the notation $g \odot X$ to indicate the image of a particular function $g$ applied to a particular domain $X$.

$$g \odot X = \{g(x), \forall x \in X | \exists g(x)\}$$

14. Let $\Sigma$ be the alphabet of the English language including numerals 0-9 and symbols $\{(, ), \sim, !, +, -, \varnothing\}$. Let $\Upsilon^*$ be the set of all words in this language. We will use $\Upsilon^*$ to label nodes and create types and subtype attributes for nodes.

## 2 STRUCTURE GRAPHS

Here, we define graph formalisms for representing BioNetGen patterns and reaction rules that are amenable to visualization.

1. A BioNetGen pattern is represented as a *pattern structure graph*, having the form $G = (V, E, \Lambda_V)$ where

$$V \subset \Upsilon^*$$
$$E \subset V \times V, \text{ unordered}$$
$$\Lambda_V = \{T_V, \Omega_V\}$$
$$T_V : V \to \{\text{mol,comp,is,bs}\}$$
$$\Omega_V : V \to \Upsilon^*$$

$T_V$ maps each node to a particular type of structural feature: molecule (mol), component (comp), internal state (is) or binding state (bs). $\Omega_V$ maps each node to a label. On binding nodes, the labels $+, -$ are used for binding states. On internal state nodes, label $\varnothing$ is used to indicate a default internal state.

Each type of node can only be adjacent to a limited number and type of neighboring nodes. The internal state can only be adjacent to one component. The bond state can only be adjacent to one or two components. In addition to exactly one internal state and one bond state, the component can be adjacent to only one molecule. The molecule itself can only be adjacent to a maximum number of each subtype of component as defined in the `molecule types` block of the model (Faeder *et al.*, 2009).

The connectivity and restrictions defined here follow from Hogg *et al.* (2014) and Lemons *et al.* (2011). The pattern as defined here is also applicable to the related rule-based frameworks of Kappa (Danos and Laneve, 2004) and Simmune (Meier-Schellersheim *et al.*, 2006).

Let $\mathbb{U}_{patt}$ denote the set of all pattern structure graphs in the model.

2. A BioNetGen reaction rule is a set of reactant patterns and a set of product patterns. Each of those patterns can be represented as a pattern structure graph. Each rule is indexed with a label derived from $\mathbb{U}_{rule} \subset \Upsilon^*$.

$$Rule = (rule, Re, Pr)$$
$$Re \subset \mathbb{U}_{patt}, Pr \subset \mathbb{U}_{patt}$$
$$rule \in \mathbb{U}_{rule}, \mathbb{U}_{rule} \subset \Upsilon^*$$

3. Given a reaction rule, each set of structure graphs is merged trivially to give the 'left' and 'right' structure graphs $G^l$ and $G^r$ respectively.

$$G^l = \bigsqcup_{\forall G \in Re} G = (V^l, E^l, \Lambda_{V^l})$$
$$G^r = \bigsqcup_{\forall G \in Pr} G = (V^r, E^r, \Lambda_{V^r})$$

4. BioNetGen computes a partial one-to-one map $\phi : V^l \nrightarrow V^r$ between reactant and product patterns. Let $dom$ and $img$ be

the subsets of $V^l$ and $V^r$ in which the map is one-to-one onto.

$$img = \phi \odot V^l$$
$$dom = \phi^{-1} \odot img$$

Note that $\phi$ refers to structures present on both sides of a reaction rule. We refer to nodes in $dom$ and $img$ as 'original' and 'duplicate' respectively.

5. To synthesize a structure graph for the rule, we merge the left and right structure graphs and remove duplicate nodes.

$$W = \{(\phi(v), v), \forall v \in dom\}$$
$$G = Del(img) \circ Map(W) \circ (G^l \sqcup G^r)$$

The resultant graph is the *rule structure graph*. It requires the additional node function prototype $side$ which keeps track of the origin of each node.

$$side_V(v) = \begin{cases} l, & v \in V^l - dom \\ r, & v \in V^r - img \\ lr, & v \in dom \end{cases}$$

Let $\mathbb{U}_{rsg}$ be the set of all rule structure graphs in the model. The rule as defined in Section 2.2 can be equivalently defined as

$$Rule = (rule, G),$$
$$rule \in \mathbb{U}_{rule}, G \in \mathbb{U}_{rsg}$$

## 3 ATOMIC PATTERNS

Here we define graph objects called atomic patterns that allow us to characterize overlaps between rules.

1. *Atomic patterns* are pattern structure graphs that represent simple classes of structural features: an internal state, a free binding site, a bond, a bond wildcard or a whole molecule (ignoring its internal structure). Let $\mathbb{U}^{atom}_{patt}$ be the set of all atomic patterns in the model. Because each atomic pattern is a pattern structure graph, $\mathbb{U}^{atom}_{patt} \subset \mathbb{U}_{patt}$.
2. Each atomic pattern is equivalently represented as an alphanumeric string with the syntax A for molecule, A(b) for free binding site, A(b∼x) for internal state, A(b!1).B(a!1) for bond and A(b!+) for bond wildcard. Because the string representation can be used to distinguish between atomic patterns, $\mathbb{U}^{atom}_{patt} \subset \Upsilon^*$ also.
3. The atomic pattern defines an *equivalence class* for isomorphic graphs. For example, using suffixes to denote vertex ids, two graphs $A_0(b_1 \sim x_2)$ and $A_3(b_4 \sim x_5)$ belong to the class of sites defined by the atomic pattern A(b∼x).
4. A vertex $v$ on a pattern structure graph can be mapped to an atomic pattern by examining its type $T_V(v)$ and its neighborhood. For example, examining the neighborhood of vertex $x_2$ in the graph $A_0(b_1 \sim x_2)$ results in mapping $x_2$ to the atomic pattern A(b∼x). For a rule structure graph, we determine this map for each of its vertices and then include it with the other node applications.

$$G = (V, E, \Lambda_V)$$
$$\theta_V : V \to \mathbb{U}^{atom}_{patt} \cup \{\varnothing\}$$
$$\theta_V \in \Lambda_V$$

The number of neighbors of each node is constrained by node type (see Section 2.1), so determining this map for each rule scales linearly with the size of the rule. Since modeled rules are typically bounded in size for a given model, determining atomic patterns from every rule in the model is $\mathcal{O}(n)$ in the number of rules.

## 4 REGULATORY GRAPHS

Here we construct regulatory graphs that are useful to represent regulatory relationships between classes of sites (atomic patterns) and reaction rules.

1. The *regulatory graph* has the form $G = (V, E, \Lambda_V, \Sigma_E)$, where

$$V \subset \Upsilon^*$$
$$E \subset V \times V, \text{unordered}$$
$$\Lambda_V = \{T_V, \Omega_V, Gr_V\}$$
$$T_V : V \to \{\text{ap,r}\}$$
$$\Omega_V : V \to \{\text{mol,fbs,wc,b,is,g},\varnothing\}$$
$$Gr_V : V \to \Upsilon^*$$
$$\Sigma_E = \{R_E, P_E, C_E, W_E\}$$
$$f_E : E \to \{0, 1\}, \forall f_E \in \Sigma_E$$

Here $T_V$ is a type map indicating the overarching type that a vertex is derived from: atomic pattern or reaction rule. $\Omega_V$ is a subtype map which is used to supplement $T_V$ indicating whether it is a molecule pattern (mol), a free binding site (fbs), a wildcard bond (wc), a bond (b), an internal state (is) or a collapsed group node (g). $Gr_V$ is used to create classes or groups of nodes. It maps each node to its assigned class name, or $\varnothing$ if unclassified. The edge functions in $\Sigma_E$ are binary partitions of the edge set for edges that satisfy a particular property, i.e. reactant ($R_E$), product ($P_E$), context ($C_E$) and wildcard ($W_E$) respectively. Multiple functions are used here because an edge can have more than one property.
2. Here we show how to transform a high resolution rule structure graph into a lower resolution regulatory graph. Consider a rule indexed by label $rule$ and its rule structure graph $G'$, as defined in Section 2.5.

$$Rule = (rule, G')$$
$$rule \in \Upsilon^*, G' \in \mathbb{U}_{rsg}$$
$$G' = (V', E', \Lambda'_{V'}),$$
$$\Lambda'_{V'} = (T'_{V'}, \Omega'_{V'}, side_{V'}, \theta_{V'})$$

As in Section 3.2, $\theta_{V'}$ maps each node to an atomic pattern. We identify which atomic pattern subgraphs are consumed,

produced or left unchanged.

$$
\begin{aligned}
V^l &= \theta_{V'} \odot \mathcal{F}(side, l) \circ V' \\
V^r &= \theta_{V'} \odot \mathcal{F}(side, r) \circ V' \\
V^{lr} &= \theta_{V'} \odot (\mathcal{F}(side, lr) \circ V' - \mathcal{F}(T, mol) \circ V')
\end{aligned}
$$

Now, we build the vertex set for the regulatory graph.

$$V = V^l \cup V^r \cup V^{lr} \cup \{rule\}$$

Note that the nodes of this graph are indexed by alphanumeric strings.

$$V \subset (\mathbb{U}_{patt}^{atom} \cup \mathbb{U}_{rule}) \subset \Upsilon^*$$

The edge set maps the rule node to each atomic pattern.

$$E = \{rule\} \times V^l \cup V^r \cup V^{lr}$$

The type map $T_V$ determines if a vertex is an atomic pattern or rule.

$$T_V(v) = \begin{cases} \text{ap}, & v \in V^l \cup V^r \cup V^{lr} \\ \text{r}, & v = rule \end{cases}$$

The edge functions identifying reactant, product and context are populated based on the set memberships.

$$
\begin{aligned}
&\forall v \in V, e \in E, s.t. v \in e, \\
&v \in V^l \iff R_E(e) = 1 \\
&v \in V^r \iff P_E(e) = 1 \\
&v \in V^{lr} \iff C_E(e) = 1
\end{aligned}
$$

The other node and edge functions are set to default values.

$$
\begin{aligned}
Gr_V &: V \to \{\varnothing\} \\
W_E &: E \to \{0\}
\end{aligned}
$$

The resultant graph $G = (V, E, \Lambda_V, \Sigma_E)$, where $\Lambda_V = \{T_V, \Omega_V, Gr_V\}$, $\Sigma_E = \{R_E, P_E, C_E, W_E\}$ is the *rule regulatory graph*.

3. Regulatory graphs can be trivially aggregated across reaction rules. Given a rule set $M$ where $G_r$ is the rule regulatory graph of each rule $r \in M$, the *full model regulatory graph* is given by

$$G_M = \bigsqcup_{r \in M} G_r$$

4. On the model regulatory graph as constructed, relationships between bond wildcards and bonds are absent and these leave crucial gaps in the signal flow. BioNetGen computes these relationships (indicated by $W$, a set of tuples) by pairwise comparison of bonds and wildcards. This is typically not expensive because bond wildcards usually form a very small percentage of the atomic patterns.

$$
\begin{aligned}
V_{wc} &= \mathcal{F}(T, \text{wc}) \circ V \\
V_b &= \mathcal{F}(T, \text{b}) \circ V \\
E' &\subset V_{wc} \times V_b
\end{aligned}
$$

First, we add edges to the graph indicating wildcard relationships.

$$
\begin{aligned}
&\forall e \in E', \\
&R_{E'}(e) = P_{E'}(e) = C_{E'}(e) = 0 \\
&W_{E'}(e) = 1 \\
&G' = (V, E \cup E', \Lambda_V, \Sigma_{E \cup E'})
\end{aligned}
$$

The graph can be left as is, or it can be *resolved* by removing all the context edges from bond wildcards and replacing them with context edges to the matched bonds. This is accomplished as follows:

$$G'' = Del(V_{wc}) \circ Map(E') \circ G'$$

Resolving the wildcard bonds is necessary to proceed to grouping nodes on the graph.

5. In the main text, we discuss how a subset of the nodes can be removed because they do not contribute to the insight of signal flow. Let $f_{bkg}$ be an arbitrary function partitioning the node set into background and foreground by assigning values 1 and 0 respectively. The simplified graph $G'$ is generated by removing background:

$$
\begin{aligned}
f_{bkg} &: V \to \{0, 1\} \\
V' &= \{v \in V | f_{bkg}(v) = 1\} \\
G' &= Del(V') \circ G
\end{aligned}
$$

6. The user can input a class assignment *seed* which maps some subset of the atomic patterns to user-defined class names.

$$
\begin{aligned}
V^{ap} &= \mathcal{F}(T_V, \text{ap}) \circ V \\
seed &: V^{ap} \to \Upsilon^* \cup \{\varnothing\}
\end{aligned}
$$

We first construct a function $\psi$ that maps each element with its assigned group, or itself if no group is assigned.

$$\psi(v) = \begin{cases} v, & seed(v) = \varnothing \\ seed(v), & seed(v) \neq \varnothing \end{cases}$$

7. We wish to use *seed* to automatically group reaction rules. Two reaction rules are defined equivalent on the reaction center (denoted by $\approx$) if they have identical sets of reactant and product relationships:

$$
\begin{aligned}
&V^{rule} = \mathcal{F}(T_V, \text{rule}) \circ V \\
&\forall v \in V^{rule}, \\
&\quad \mathcal{R}(v) = \{\psi(v'), \forall v' \in V^{ap} | R_E((v, v')) = 1\} \\
&\quad \mathcal{P}(v) = \{\psi(v'), \forall v' \in V^{ap} | P_E((v, v')) = 1\} \\
&v \approx v' \iff \\
&\quad \mathcal{R}(v) = \mathcal{R}(v'), \\
&\quad \mathcal{P}(v) = \mathcal{P}(v')
\end{aligned}
$$

The new grouping $Gr_V$ retains the *seed* grouping of atomic patterns and assigns a unique class name to reaction rules equivalent on the reaction center.

$$\begin{aligned}
&\forall v \in V^{ap},\\
&\quad Gr_V(v) = seed(v)\\
&\forall v, v' \in V^{rule},\\
&\quad v \approx v' \iff Gr_V(v) = Gr_V(v')\\
&\quad v \not\approx v' \iff Gr_V(v) \neq Gr_V(v')
\end{aligned}$$

The grouping process has $\mathcal{O}(n * m \log m)$ time complexity where $n$ is the number of rules and $m$ is the number of atomic patterns that participate in a reaction center. For typical systems, this amounts to being $\mathcal{O}(n)$, since the size of the reaction center is bounded. The exception is when the model has many synthesis and deletion reaction rules that use large complex patterns.

8. The complexity of the graph can be reduced by rendering the grouped nodes indistinguishable from each other. First, each group name is added as a separate node. Then edges are remapped to the group names and individual group members are deleted.

$$\begin{aligned}
dom &= \{v \in V | Gr_V(v) \neq \varnothing\}\\
img &= Gr_V \odot dom\\
T_{img}(Gr_V(v)) &= T_V(v), \forall v \in dom\\
\Omega_{img}(v) &= \text{g}, \forall v \in img\\
G' &= (img, \{\}, \{T_{img}, \Omega_{img}\}, \{\})\\
Y &= \{(v, Gr_V(v)) \forall v \in dom\}\\
G'' &= Del(dom) \circ Map(Y) \circ (G \sqcup G')
\end{aligned}$$

The resultant graph is the *reduced regulatory graph*.

## 5 VISUAL CONVENTIONS

Here we provide appropriate transformations to generate a visual object from the graph types defined above,

1. **Site Graphs** Given a pattern structure graph as in Section 2.1 above:

   a. Nest component nodes within adjacent molecule node.
   b. Nest internal state nodes within adjacent component node.
   c. Remove unbound state nodes.
   d. Identify parent components of bond node. Remove bond node. Add edge between parents.

2. **Direct Rule Visualization** Given a reaction rule defined using reactant and product patterns, as in Section 2.2 above,

   a. Draw a node to represent the rule.
   b. Draw a separate node to represent each pattern.
   c. Within each pattern node, embed the respective site graph.
   d. Draw a directed edge from each reactant pattern to the rule.
   e. Draw a directed edge from the rule to each product pattern.

3. **Compact Rule Visualization** Given a rule structure graph as in Section 2.5 above,

   a. Partition the set of nodes using the $side$ and $type$ functions.
   b. For molecule nodes with side $l$ or $r$,

      (1) Draw a graph operation node named DeleteMol if side is $l$ or AddMol if side is $r$.
      (2) Draw a directed edge between the molecule and the graph operation node. The edge direction is toward the graph operation node if DeleteMol and away if AddMol.

   c. For internal states with side $l$ or $r$,

      (1) Ignore if side of parent component is $l$ or $r$.
      (2) Partition by parent component.
      (3) Add a graph operation node named ChangeState adjacent to each parent component.
      (4) Draw a directed edge from each internal state to the ChangeState node for its respective parent component. The edge direction is toward the graph operation node if side is $l$ and away if side is $r$.

   d. For bonds with side $l$ or $r$,

      (1) Replace with graph operation node named DeleteBond if $l$ and AddBond if $r$.
      (2) Add edge direction on incident edges: toward the graph operation node if DeleteBond and away if DeleteBond.

   e. Apply site graph conventions on all molecule, component and internal state nodes.
   f. Nest ChangeState operation nodes within adjacent components.

4. **Regulatory Graph** Given a regulatory graph as defined in Section 4.1 above,

   a. Draw a node for each reaction rule and atomic pattern. For collapsed graphs, the $type$ function still defines nodes as reaction rule and atomic pattern, so the same conventions apply.
   b. The set of edge functions define reactant, product, context and wildcard relations on the nodes. For each valid relation, draw an edge between the corresponding nodes, allowing parallel edges to exist. The edge direction is

      - Toward the rule node if a reactant or context relation.
      - Away from the rule node if a product relation.
      - Toward the wildcard node if a wildcard relation.

      The edge color is a light color if a context relation and a dark color otherwise.

c. If a grouping is defined as in Section 4.7,

(1) Draw a node for each group.
(2) Nest members of a group within the group node.

## 6 FIGURES AND TABLES

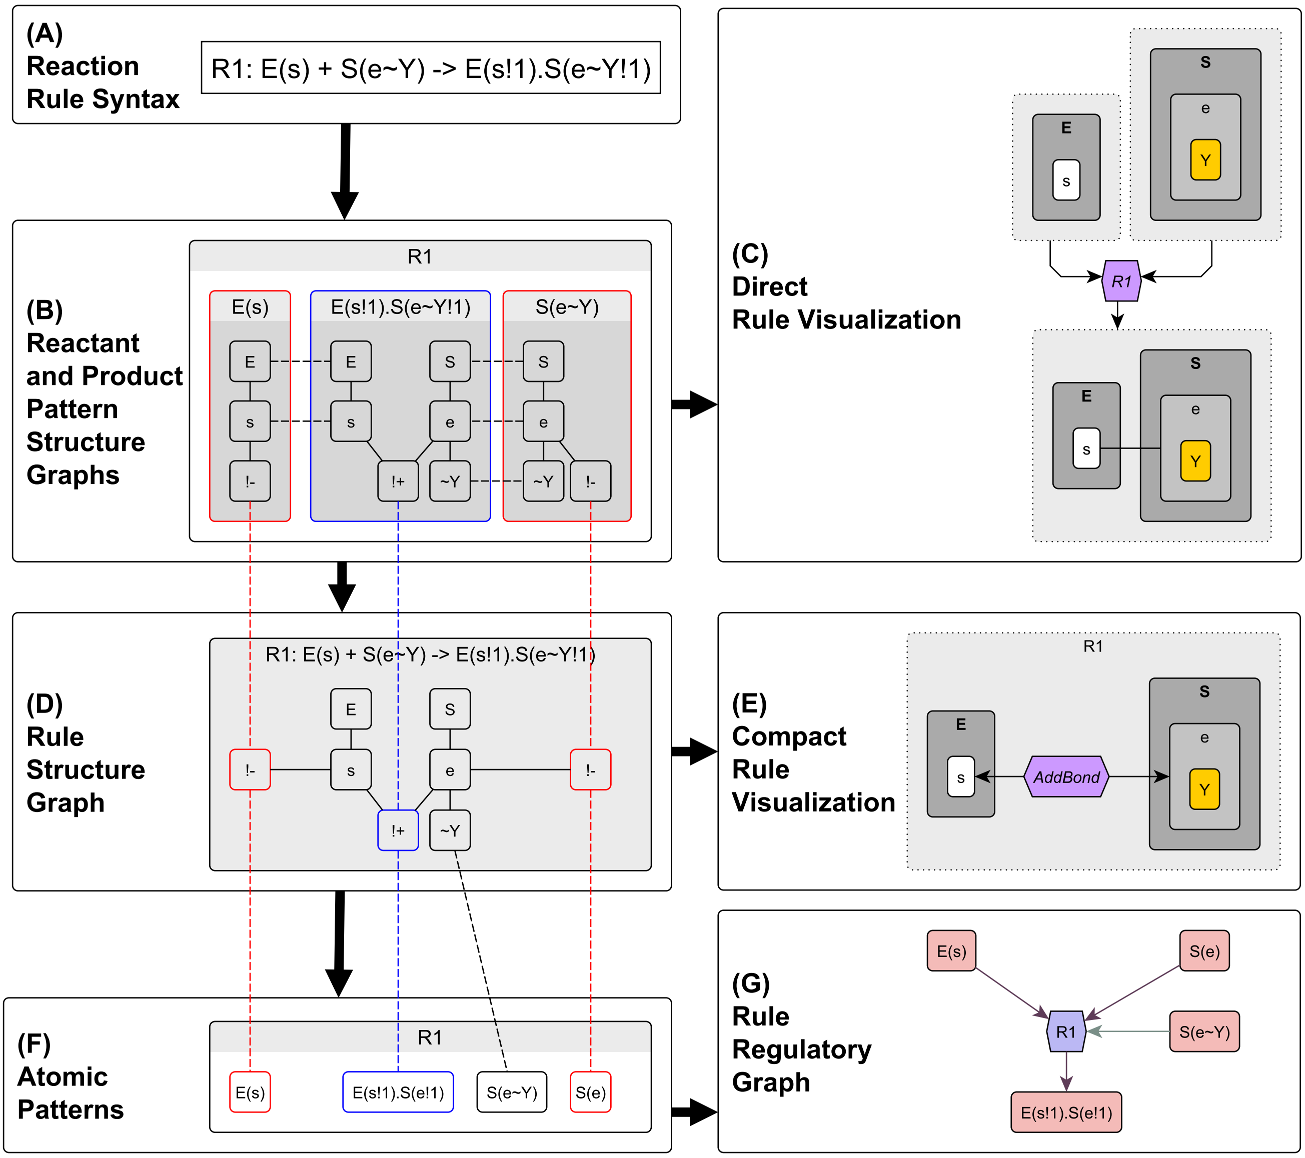


**Fig. S1:** Summary of relationships between graph abstractions. (A) A reaction rule R1 has reactant patterns `E(s)`, `S(e~Y)` and product pattern `E(s!1).S(e~Y)`. (B) Patterns are transformed into structure graphs where each molecule, component, internal state and bond state is a node and edges represent hierarchical relations. Derived from the pattern definition in Hogg *et al.* (2014) (Supplement). Compare with hierarchical graphs in Lemons *et al.* (2011). (C) Pattern structure graphs are transformed into site graphs. Embedding site graphs in the nodes of a bipartite graph enables direct rule visualization. Compare with Simmune Modeler (Zhang *et al.*, 2013) and SBGN Process Description (Le Novère *et al.*, 2009). (D) BioNetGen computes a correspondence between reactant and product patterns. This is used to merge the pattern structure graphs into a single rule structure graph, while keeping track of whether nodes are from reactant (red), product (blue) or both (black). (E) The rule structure graph is transformed into a compact rule visualization. (F) Examining the neighborhood of individual nodes, we can identify instances of atomic pattern subgraphs. The source of the atomic pattern (reactant/product/both) is inherited from the node. (G) Relationships between atomic patterns and the rule are visualized as a regulatory graph. Dark edges incoming and outgoing on the rule node indicate reactant and product relationships respectively and light edges indicate context relationships. Compare with Rxncon regulatory graph (Tiger *et al.*, 2012).

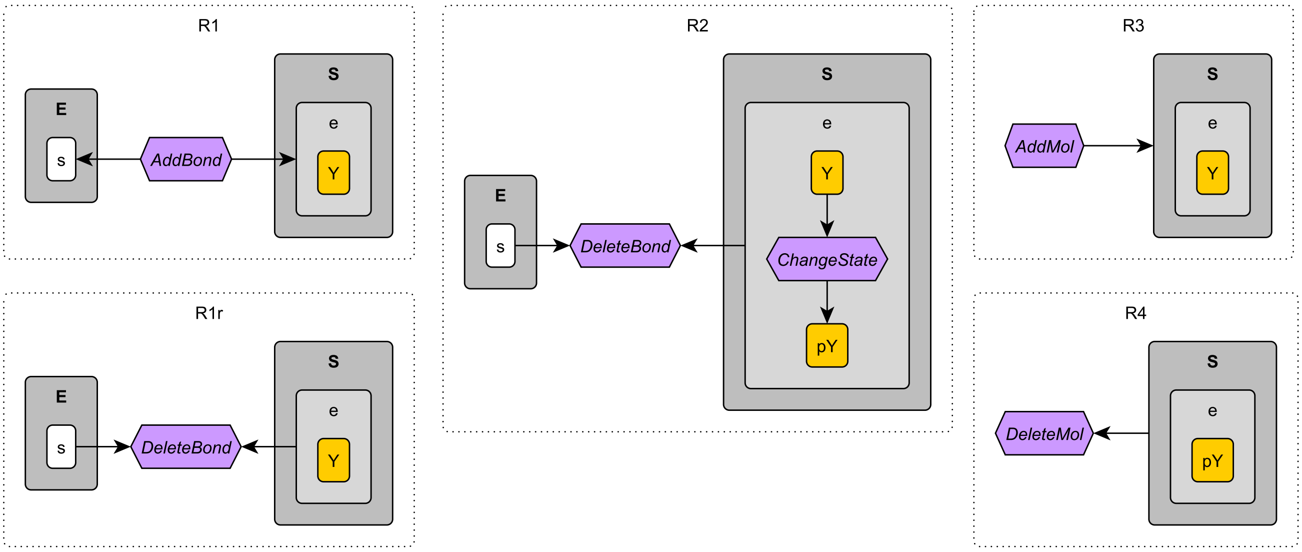


**Fig. S2:** Supported graph operations in compact rule visualization include AddBond, DeleteBond, AddMol, DeleteMol and ChangeState. A rule might have more than one operation happen simultaneously, e.g. R2 models simultaneous dissociation and phosphorylation.

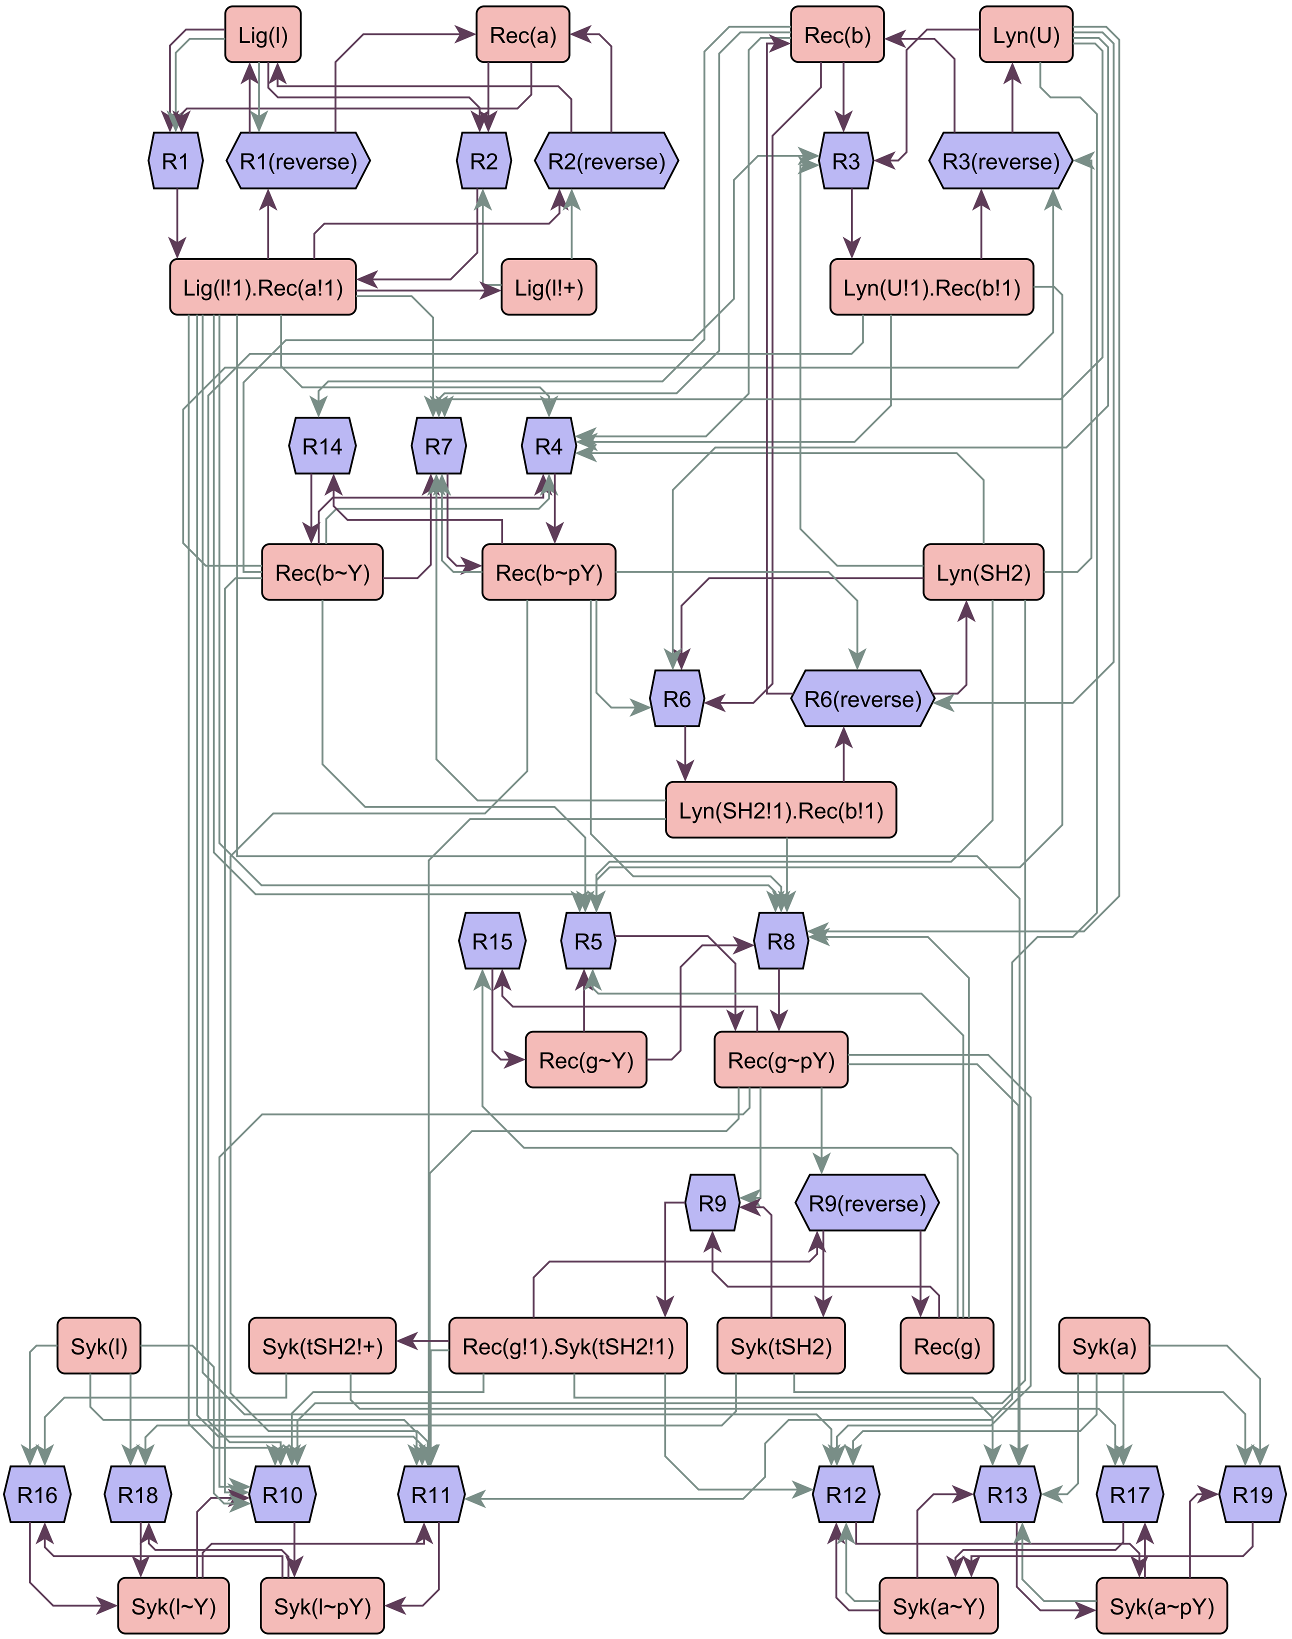


**Fig. S3:** Full regulatory graph of the Faeder *et al.* (2003) model of signaling from the Fc$\varepsilon$RI receptor.

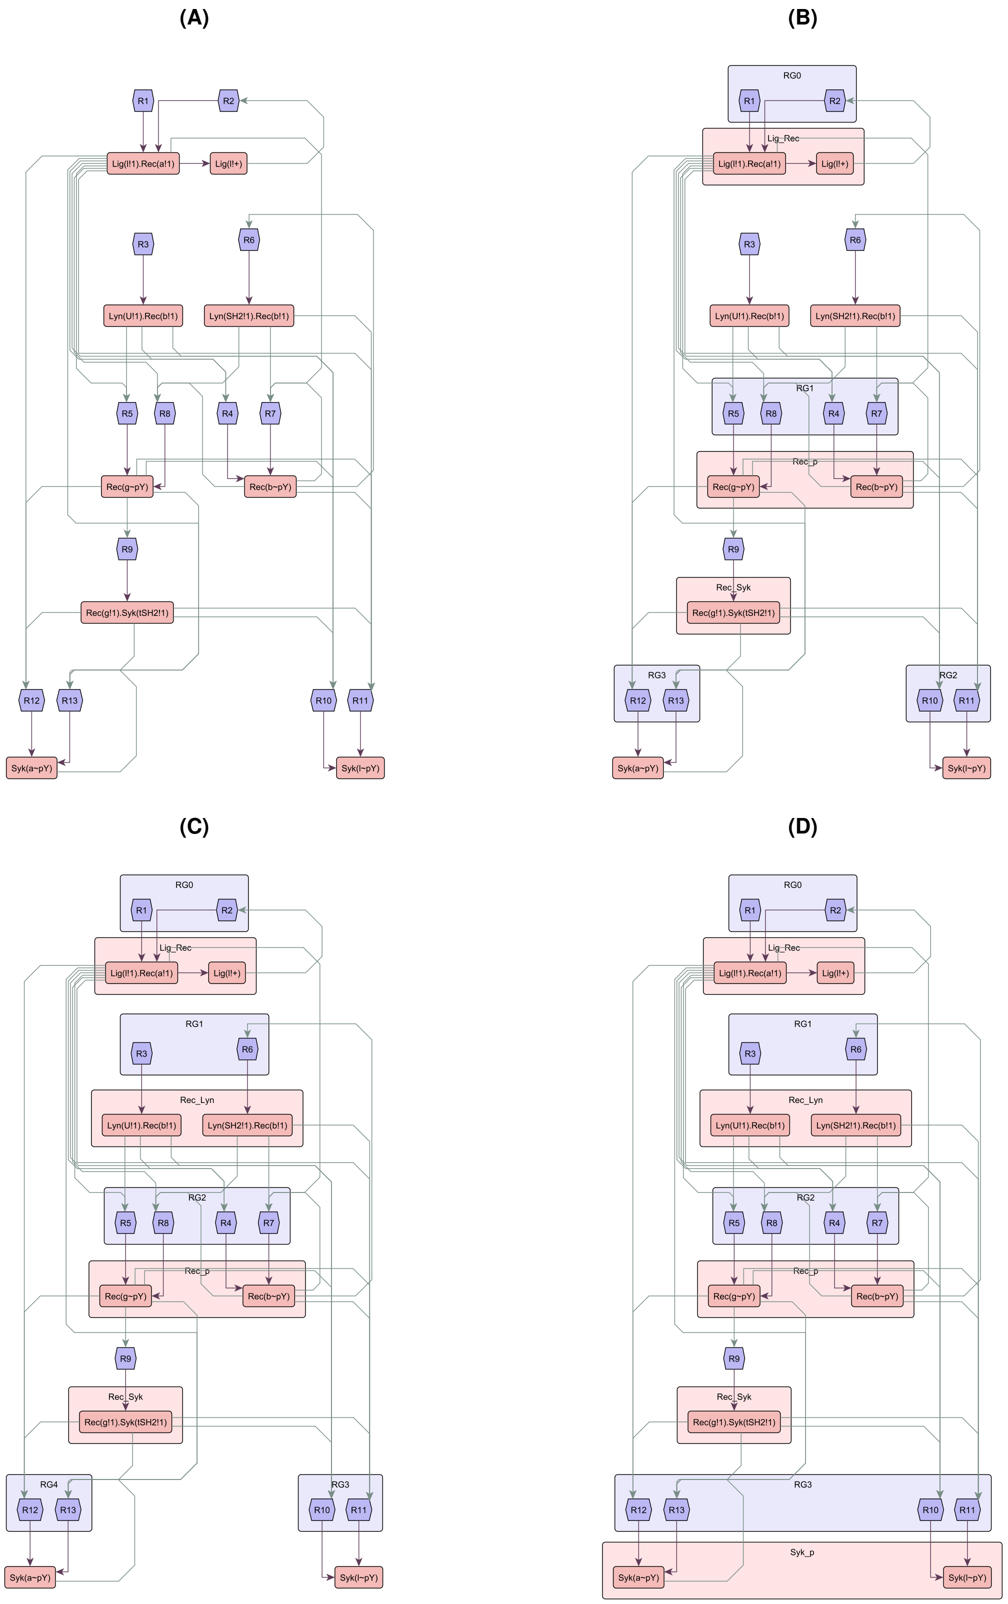


**Fig. S4:** Different grouping strategies applied to the Faeder *et al.* (2003) model regulatory graph. (A) Regulatory graph with background nodes removed and no grouping performed. (B) Both Lyn-receptor binding states and both Syk phosphorylation sites are ungrouped. (C) The Lyn-receptor binding states were grouped under Rec_Lyn. (D) The Syk phosphorylation sites were grouped under Syk_p. The collapsed versions of Panels B-D are used in the main text.

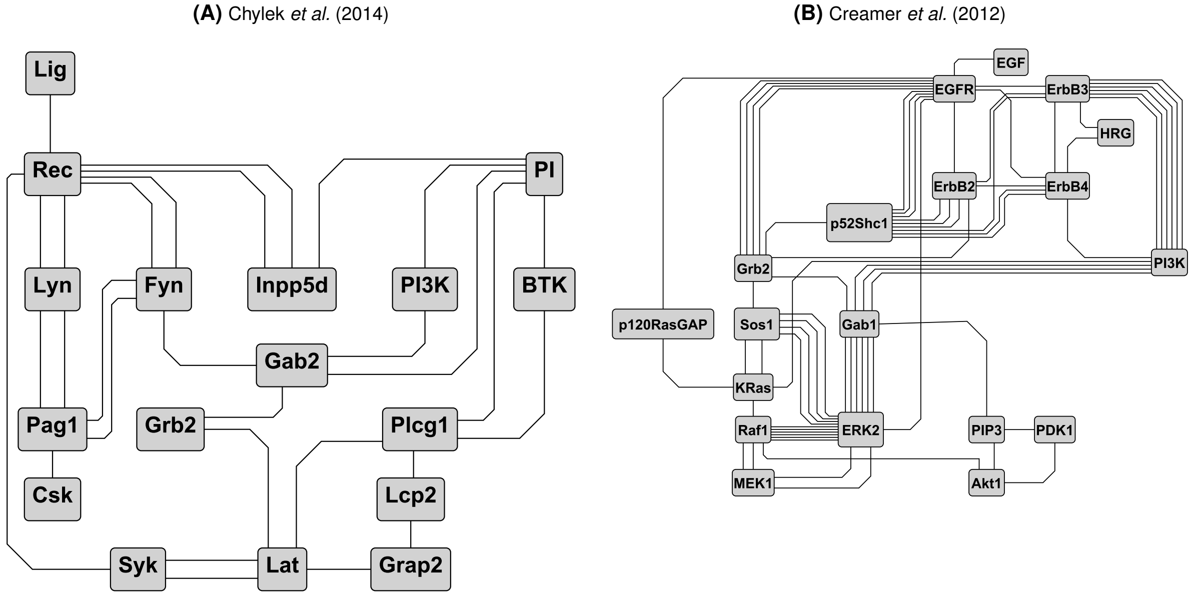


**Fig. S5:** Compressed contact maps of the Chylek *et al.* (2014) and Creamer *et al.* (2012). Because these are large models, we have hidden the components and internal states away to only show molecules and number of pairwise-bonds that are possible.

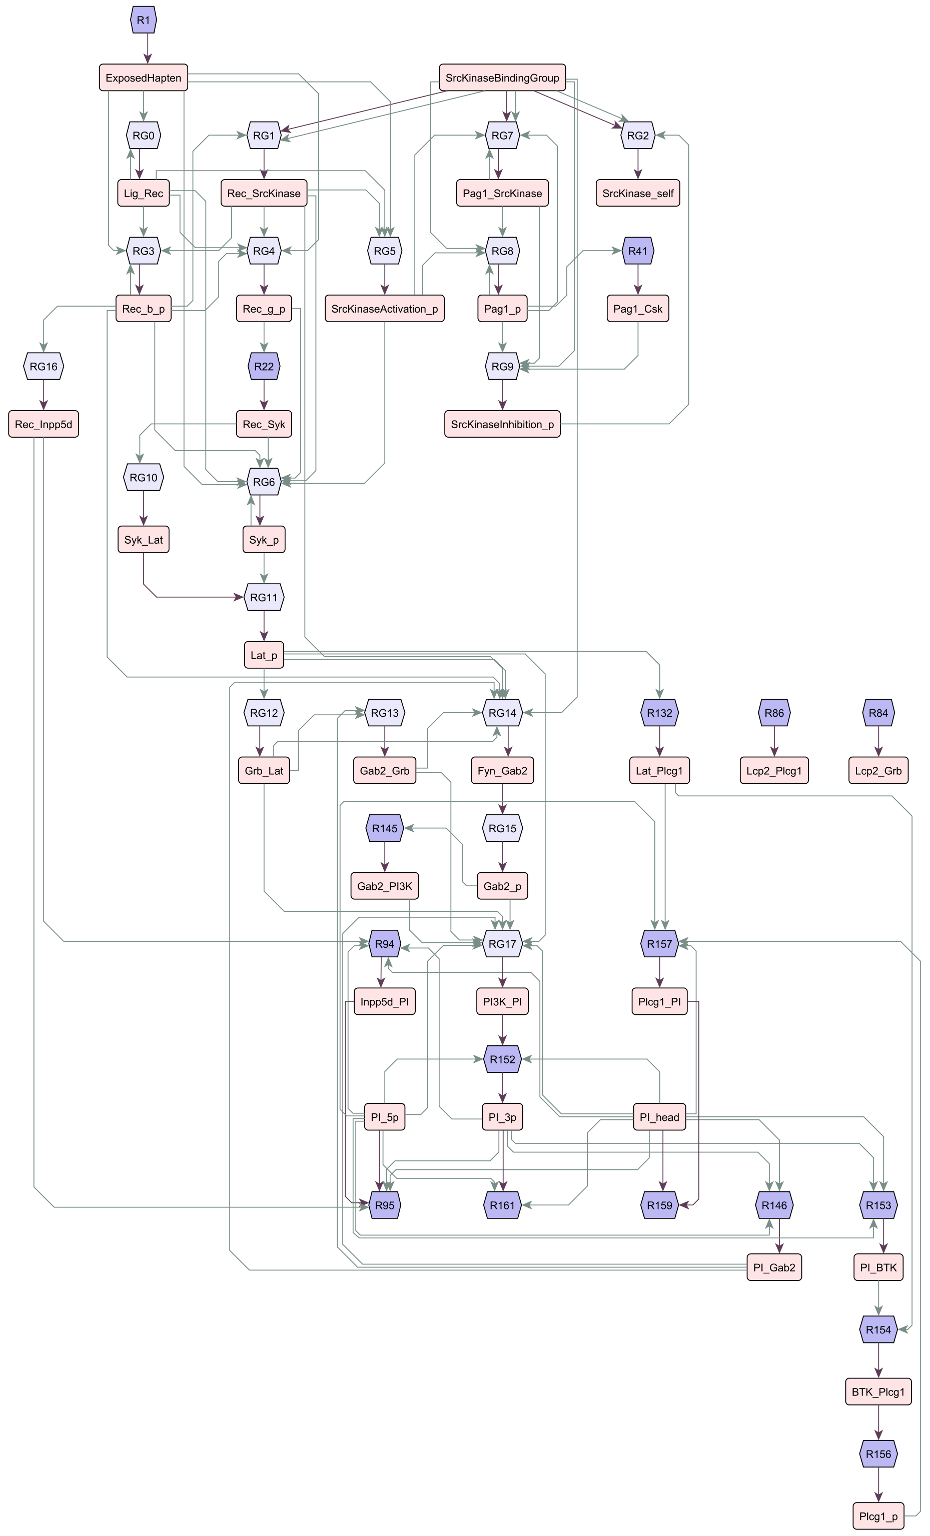


**Fig. S6:** Regulatory graph of the Chylek *et al.* (2014) library of signaling from the Fc$\varepsilon$RI receptor.

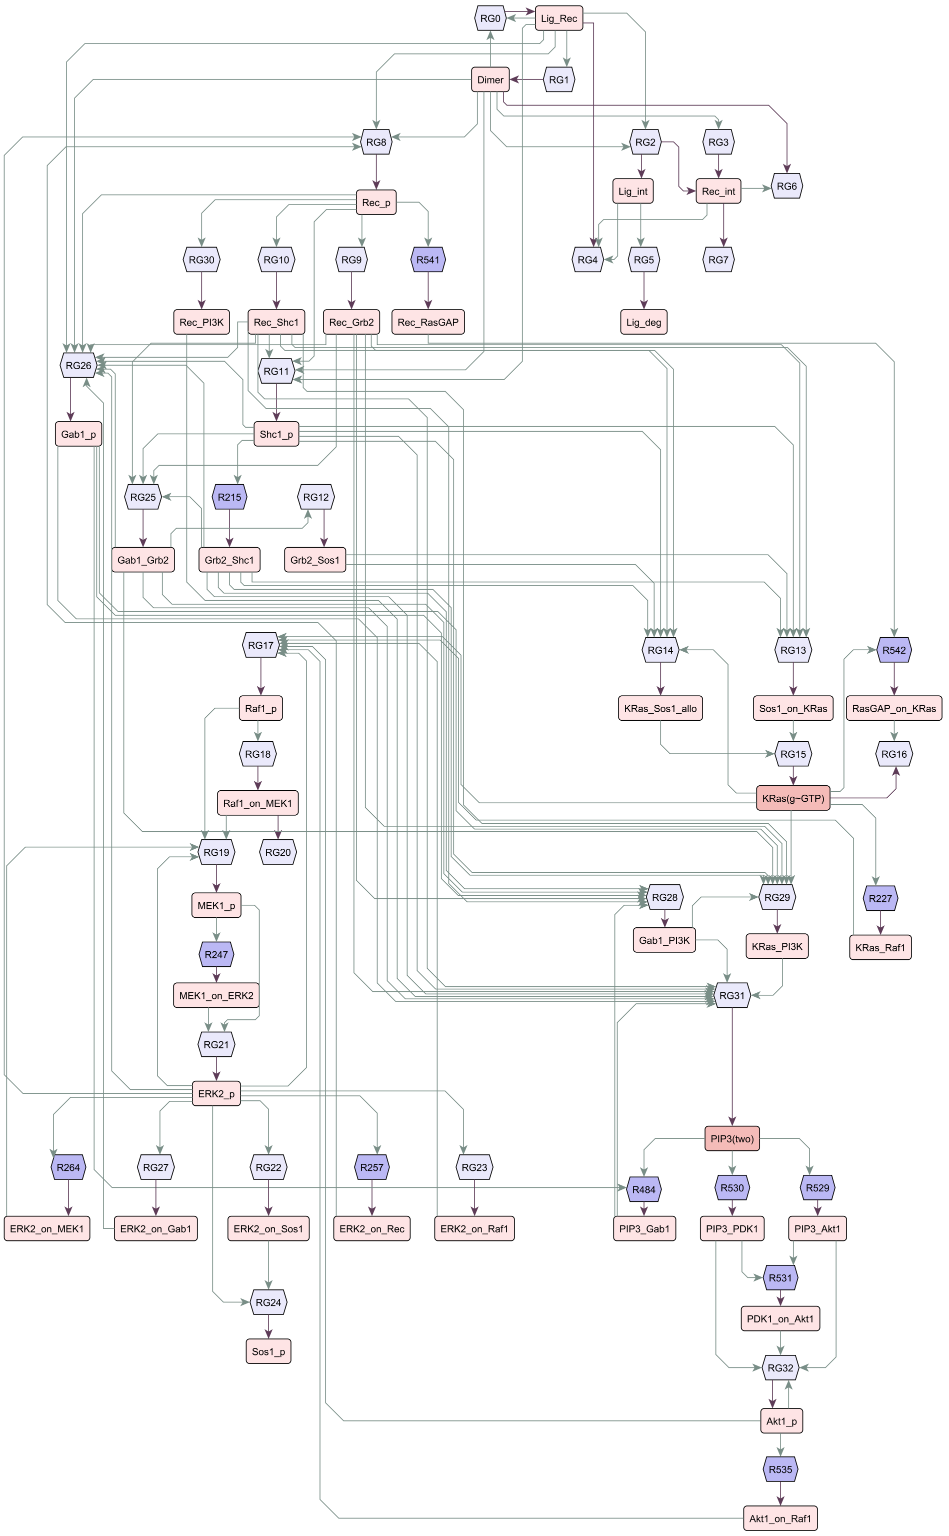


**Fig. S7:** Regulatory graph of the Creamer *et al.* (2012) model of signaling from the ErbB family of receptors.

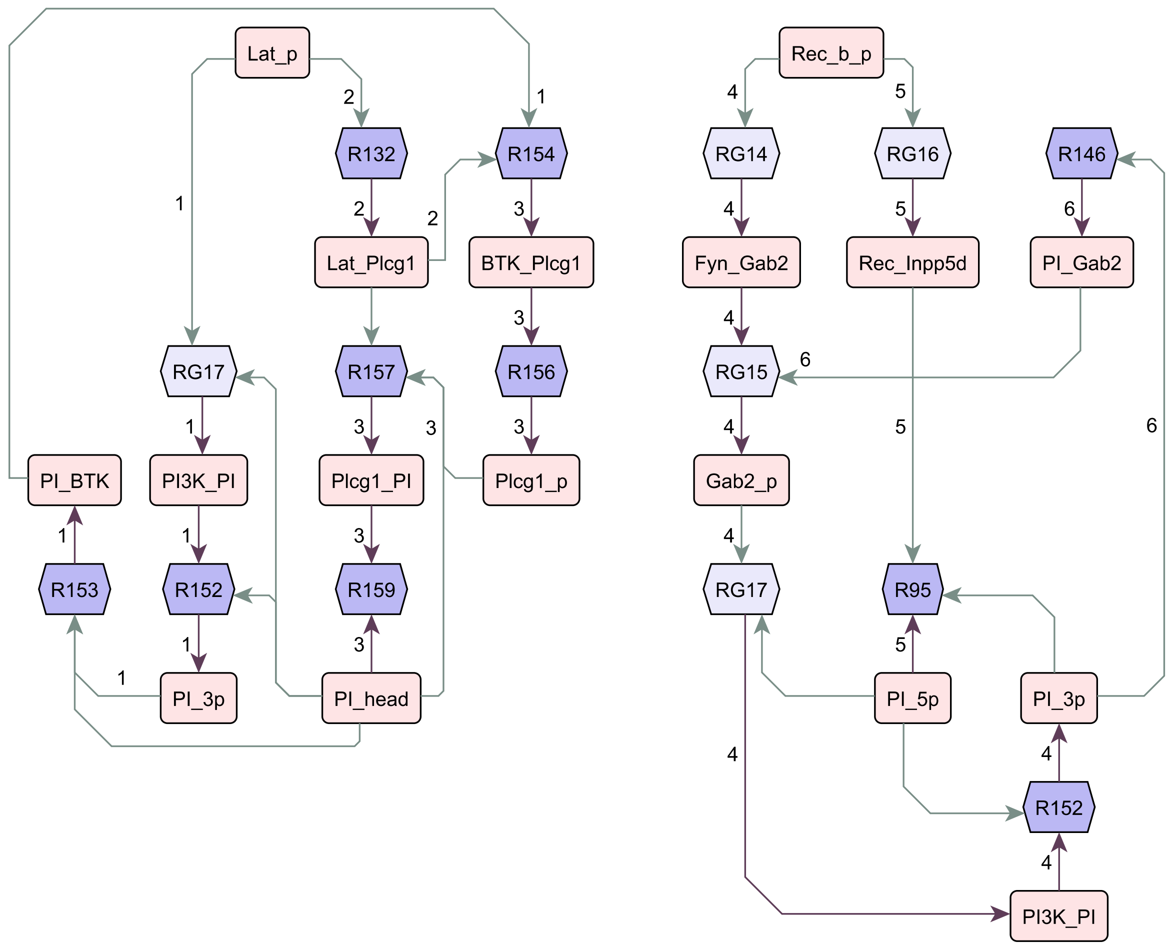


**Fig. S8:** Network motifs in the Chylek *et al.* (2014) library and their representation on the regulatory graph. In this model, PIP3 was treated as a structured molecule, therefore the nodes PI_3p and PI_5p represent phosphate at the 3'-OH and 5'-OH of the phosphoinositol molecule respectively and PI_head represents the uncleaved phosphoinositol headgroup. On the graph, R152 is seen to produce PI_3p and represents kinase activity by PI3K. R95 is seen to consume PI_5p and represents phosphatase activity by Inpp5d. R159 is seen to consume PI_head and represents phospholipid cleavage by Plcg1. (A) Cascades 1 and 2 both start with phosphorylated Lat. Cascade 1 shows PI3K activity, followed by recruitment of BTK to the membrane. Cascade 2 shows Plcg1 recruitment. Both cascades converge on activation of Plcg1 by BTK, resulting in a coherent feed-forward loop. (B) Cascades 4 and 5 both start with phosphorylated receptor. Cascade 4 shows Gab2 phosphorylation leading to PI3K activity which increases PIP3 concentration. Cascade 5 follows recruitment of Inpp5d to receptor leading to phosphatase activity that decreases PIP3 concentration. Cascades 4 and 5 together constitute an incoherent feed-forward loop. Cascade 6 depicts increased Gab2 recruitment to the membrane due to PIP3 binding leading to Gab2 phosphorylation. Cascades 4 and 6 together constitute a positive feedback loop.

| Model | Rules | Nodes or Entities | | | | | |
|---|---|---|---|---|---|---|---|
| | | cmap | rbm | reg | reg2 | rinf | rxn |
| Faeder2003 | 24 | 25 | 304 | 47 | 15 | 24 | 4034 |
| Kocieniewski2012 | 28 | 28 | 279 | 52 | | 28 | 572 |
| Blinov2006 | 39 | 27 | 414 | 65 | | 39 | 4105 |
| Barua2007 | 43 | 17 | 595 | 61 | | 43 | 1181 |
| Nag2009 | 52 | 38 | 706 | 86 | | 52 | 13660 |
| Thomson2011 | 54 | 44 | 570 | 98 | | 54 | 2041 |
| Barua2012 | 86 | 60 | 884 | 144 | | 86 | 25510 |
| Dushek2011 | 128 | 34 | 1320 | 161 | | 128 | 427 |
| Chylek2014 | 178 | 144 | 2152 | 313 | 70 | 178 | |
| Creamer2012 | 625 | 345 | 11392 | 939 | 85 | 625 | |

| Model | Rules | Edges or Entity Relations | | | | | |
|---|---|---|---|---|---|---|---|
| | | cmap | rbm | reg | reg2 | rinf | rxn |
| Faeder2003 | 24 | 25 | 340 | 128 | 25 | 162 | 10016 |
| Kocieniewski2012 | 28 | 27 | 279 | 171 | | 133 | 1274 |
| Blinov2006 | 39 | 28 | 422 | 212 | | 536 | 10498 |
| Barua2007 | 43 | 18 | 611 | 342 | | 1054 | 2568 |
| Nag2009 | 52 | 38 | 765 | 298 | | 627 | 35168 |
| Thomson2011 | 54 | 43 | 615 | 310 | | 374 | 4796 |
| Barua2012 | 86 | 66 | 918 | 527 | | 1082 | 84782 |
| Dushek2011 | 128 | 35 | 1372 | 974 | | 4676 | 568 |
| Chylek2014 | 178 | 156 | 2326 | 1084 | 129 | 1864 | |
| Creamer2012 | 625 | 398 | 12992 | 5110 | 157 | 21754 | |

| Model | Number of nodes (fold-difference) | | | | Edge-to-node ratio (fold-difference) | | | |
|---|---|---|---|---|---|---|---|---|
| | reg/cmap | reg2/cmap | reg/rinf | reg2/rinf | reg/cmap | reg2/cmap | reg/rinf | reg2/rinf |
| Faeder2003 | 1.88 | 0.60 | 1.96 | 0.63 | 2.72 | 1.67 | 0.40 | 0.25 |
| Kocieniewski2012 | 1.86 | | 1.86 | | 3.41 | | 0.69 | |
| Blinov2006 | 2.41 | | 1.67 | | 3.15 | | 0.24 | |
| Barua2007 | 3.59 | | 1.42 | | 5.30 | | 0.23 | |
| Nag2009 | 2.26 | | 1.65 | | 3.47 | | 0.29 | |
| Thomson2011 | 2.23 | | 1.81 | | 3.24 | | 0.46 | |
| Barua2012 | 2.40 | | 1.67 | | 3.33 | | 0.29 | |
| Dushek2011 | 4.74 | | 1.26 | | 5.88 | | 0.17 | |
| Chylek2014 | 2.17 | 0.49 | 1.76 | 0.39 | 3.20 | 1.70 | 0.33 | 0.18 |
| Creamer2012 | 2.72 | 0.25 | 1.50 | 0.14 | 4.72 | 1.60 | 0.16 | 0.05 |

**Fig. S9:** Statistics of diagrams of ten models from the literature (Faeder *et al.*, 2003; Kocieniewski *et al.*, 2012; Blinov *et al.*, 2006; Barua *et al.*, 2007; Nag *et al.*, 2009; Thomson *et al.*, 2011; Barua *et al.*, 2012; Dushek *et al.*, 2011; Chylek *et al.*, 2014; Creamer *et al.*, 2012). cmap = Contact Map (Danos *et al.*, 2012), rbm = Rule-based models with rules visualized using compact rule visualization, reg = Full regulatory graph, reg2 = Reduced regulatory graph that incorporates expert input, rinf = Rule influence diagram (Smith *et al.*, 2012), rxn = Reaction network. When site graphs are present, we counted bonds as nodes and relationships between bonds and components as edges.

# REFERENCES


Barua, D., Faeder, J. R., and Haugh, J. M. (2007). Structure-based kinetic models of modular signaling protein function: focus on Shp2. *Biophysical journal*, **92**(7), 2290–300.

Barua, D., Hlavacek, W. S., and Lipniacki, T. (2012). A computational model for early events in B cell antigen receptor signaling: analysis of the roles of Lyn and Fyn. *Journal of immunology (Baltimore, Md. : 1950)*, **189**(2), 646–58.

Blinov, M. L., Faeder, J. R., Goldstein, B., and Hlavacek, W. S. (2006). A network model of early events in epidermal growth factor receptor signaling that accounts for combinatorial complexity. *Bio Systems*, **83**(2-3), 136–51.

Chylek, L. A., Holowka, D. A., Baird, B. A., and Hlavacek, W. S. (2014). An Interaction Library for the Fc$\epsilon$RI Signaling Network. *Frontiers in immunology*, **5**, 172.

Creamer, M. S., Stites, E. C., Aziz, M., Cahill, J. a., Tan, C. W., Berens, M. E., Han, H., Bussey, K. J., Von Hoff, D. D., Hlavacek, W. S., and Posner, R. G. (2012). Specification, annotation, visualization and simulation of a large rule-based model for ERBB receptor signaling. *BMC systems biology*, **6**(1), 107.

Danos, V. and Laneve, C. (2004). Formal molecular biology. In *Theoretical Computer Science*, volume 325, pages 69–110.

Danos, V., Feret, J., Fontana, W., Harmer, R., Hayman, J., Krivine, J., Thompson-Walsh, C., and Winskel, G. (2012). Graphs, Rewriting and Pathway Reconstruction for Rule-Based Models. In D. D'Souza, T. Kavitha, and J. Radhakrishnan, editors, *IARCS Annual Conference on Foundations of Software Technology and Theoretical Computer Science (FSTTCS 2012)*, volume 18 of *Leibniz International Proceedings in Informatics (LIPIcs)*, pages 276–288, Dagstuhl, Germany. Schloss Dagstuhl–Leibniz-Zentrum fuer Informatik.

Dushek, O., Van Der Merwe, P. A., and Shahrezaei, V. (2011). Ultrasensitivity in multisite phosphorylation of membrane-anchored proteins. *Biophysical Journal*, **100**(5), 1189–1197.

Faeder, J. R., Hlavacek, W. S., Reischl, I., Blinov, M. L., Metzger, H., Redondo, A., Wofsy, C., and Goldstein, B. (2003). Investigation of early events in Fc epsilon RI-mediated signaling using a detailed mathematical model. *Journal of immunology (Baltimore, Md. : 1950)*, **170**(7), 3769–81.

Faeder, J. R., Blinov, M. L., and Hlavacek, W. S. (2009). Rule-based modeling of biochemical systems with BioNetGen. *Methods in molecular biology (Clifton, N.J.)*, **500**(2), 113–67.

Hogg, J. S., Harris, L. A., Stover, L. J., Nair, N. S., and Faeder, J. R. (2014). Exact hybrid particle/population simulation of rule-based models of biochemical systems. *PLoS computational biology*, **10**(4), e1003544.

Kocieniewski, P., Faeder, J. R., and Lipniacki, T. (2012). The interplay of double phosphorylation and scaffolding in MAPK pathways. *Journal of theoretical biology*, **295**, 116–24.

Le Novère, N., Hucka, M., Mi, H., Moodie, S., Schreiber, F., Sorokin, A., Demir, E., Wegner, K., Aladjem, M. I., Wimalaratne, S. M., Bergman, F. T., Gauges, R., Ghazal, P., Kawaji, H., Li, L., Matsuoka, Y., Villéger, A., Boyd, S. E., Calzone, L., Courtot, M., Dogrusoz, U., Freeman, T. C., Funahashi, A., Ghosh, S., Jouraku, A., Kim, S., Kolpakov, F., Luna, A., Sahle, S., Schmidt, E., Watterson, S., Wu, G., Goryanin, I., Kell, D. B., Sander, C., Sauro, H., Snoep, J. L., Kohn, K., and Kitano, H. (2009). The Systems Biology Graphical Notation. *Nature biotechnology*, **27**(8), 735–41.

Lemons, N. W., Hu, B., and Hlavacek, W. S. (2011). Hierarchical graphs for rule-based modeling of biochemical systems. *BMC bioinformatics*, **12**, 45.

Meier-Schellersheim, M., Xu, X., Angermann, B., Kunkel, E. J., Jin, T., and Germain, R. N. (2006). Key role of local regulation in chemosensing revealed by a new molecular interaction-based modeling method. *PLoS Computational Biology*, **2**, 0710–0724.

Nag, A., Monine, M. I., Faeder, J. R., and Goldstein, B. (2009). Aggregation of membrane proteins by cytosolic cross-linkers: theory and simulation of the LAT-Grb2-SOS1 system. *Biophysical journal*, **96**(7), 2604–23.

Smith, A. M., Xu, W., Sun, Y., Faeder, J. R., and Marai, G. E. (2012). RuleBender: integrated modeling, simulation and visualization for rule-based intracellular biochemistry. *BMC bioinformatics*, **13 Suppl 8**, S3.

Thomson, T. M., Benjamin, K. R., Bush, A., Love, T., Pincus, D., Resnekov, O., Yu, R. C., Gordon, A., Colman-Lerner, A., Endy, D., and Brent, R. (2011). Scaffold number in yeast signaling system sets tradeoff between system output and dynamic range. *Proceedings of the National Academy of Sciences*, **108**(50), 20265–20270.

Tiger, C.-F., Krause, F., Cedersund, G., Palmér, R., Klipp, E., Hohmann, S., Kitano, H., and Krantz, M. (2012). A framework for mapping, visualisation and automatic model creation of signal-transduction networks. *Molecular systems biology*, **8**(578), 578.

Zhang, F., Angermann, B. R., and Meier-Schellersheim, M. (2013). The Simmune Modeler visual interface for creating signaling networks based on bi-molecular interactions. *Bioinformatics (Oxford, England)*, **29**(9), 1229–30.
